# Supplementary material for: Gain/Loss-free Non-Hermitian Metamaterials
Source: arXiv:2408.16290 source file (2025-04-21)
Supplement: Supplementary file 1 [file SM.pdf]

# Gain/Loss-free Non-Hermitian Metamaterials

Maopeng Wu,[1,*] Mingze Weng,[1,*] Zhonghai Chi,[2] Siyong Zheng,[2] Fubei Liu,[2] Weijia Luo,[2] Qian Zhao,[1,†] Yonggang Meng,[1] and Ji Zhou[2,‡]
[1]*State Key Laboratory of Tribology in Advanced Equipment, Department of Mechanical Engineering, Tsinghua University, Beijing 100084, China*
[2]*State Key Laboratory of New Ceramics and Fine Processing, School of Materials Science and Engineering, Tsinghua University, Beijing 100084, China*
(Dated: April 21, 2025)

## CONTENTS


- I. A review about self-energy 1
  - A. Junction 1
  - B. Reservoir argument 1
- II. Edge state Hamiltonian 2
  - A. Green's function with periodic boundaries 3
  - B. Hopping perturbation 3
  - C. Green's function with the perturbation 3
  - D. Edge state wave vector 4
- III. Self-energy 4
- IV. Response profile 5
- V. Realization of the hopping with a phase 6
  - A. Ill-defined admittance of microwave circulators 6
  - B. Review of signal flow graphs 7
  - C. Two sites 8
  - D. Three sites 8
  - E. Four sites 9
- VI. Simulations of microstrip line metamaterials 10
  - A. Upgrade of TTCs 10
  - B. ML Haldane model 11
  - C. Field-circuit co-simulation of the junction 12
- VII. Kwant simulation 13
  - A. Topological junction 14
  - B. Imaginary absorbing potential 14
- VIII. Experimental details 14
  - A. Circuit realization of Haldane model 15
  - B. Circuit realization of the semi-infinite conductor 15
  - C. Measuring of the non-Bloch transport 15
- References 15



* These two authors contributed equally.
† zhaoqian@tsinghua.edu.cn
‡ zhouji@tsinghua.edu.cn


## I. A REVIEW ABOUT SELF-ENERGY

### A. Junction

Let us first give the topological junction an intuition. Assuming each side of the junction is described by a Hermitian Hamiltonian, $H_0$ and $H_e$, and the two sides are coupled through some surface mechanism, such as the chemical bonds. Then the junction is Hermitian and the total Hamiltonian can be written as.

$$H_J = \begin{pmatrix} H_0 & C \\ C^\dagger & H_e \end{pmatrix}, \tag{1}$$

where $C$ denotes the coupling. Correspondingly, the retarded green function $G_J$ can be defined as $G_j = (E + i0^+ - H_J)^{-1}$ or

$$G_J = \begin{pmatrix} G_0 & G_{0e} \\ G_{e0} & G_e \end{pmatrix}. \tag{2}$$

When one of the sides is so "large", say the side described by $H_e$, that the effect of $H_0$ on $H_e$ is negligible. In this case, $H_e$ constitutes a reservoir or the environment. After some simple algebra, we can find the Green's function $G_0$ of the smaller side is expressed as $G_0 = E + i0^+ - H_0 - \Sigma$, where $\Sigma = C^\dagger G_e^{-1} C$ is the so called self-energy and the effect of $H_e$ on $H_0$ is encoded with it. So the effective Hamiltonian $H_{\text{eff}}$ of the smaller side is $H_{\text{eff}} = H_0 + \Sigma$, and in general $H_{\text{eff}}$ is non-Hermitian $H_{\text{eff}} \neq H_{\text{eff}}^\dagger$ owing to the complexity of $\Sigma$. Note that the non-Hermitisity is introduced without any gain or loss, while the gain and loss are essential in optical realization. The concept of self-energy is widely applied in physics, such as those coming from the electron-electron/phonon Coulomb interactions, the impurity scattering and the interaction with the reservoir (considered here), although their physical origins may differ.

### B. Reservoir argument

In the main article, we realize an effective NH system by considering two coupled subsystems. The self-energy treatment requires that one of the subsystems can be viewed as the reservoir. Here we show that self-energy is out of the capability to delineate two comparable coupled subsystems.

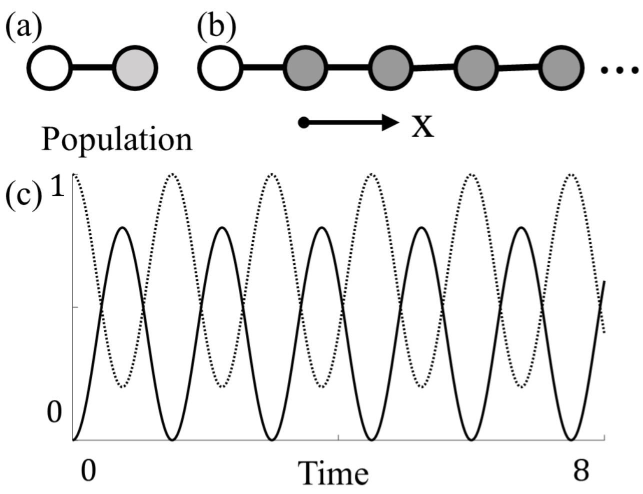


FIG. 1. Reservoir argument. (a) Two comparable coupled subsystems I and II. (b) Two coupled subsystems with the subsystem II consisting of $N$ states. (c) The population dynamics as a function of time in two comparable coupled subsystems. $E_1 = 0$, $E_2 = 1$ and $\Omega = 1$. The solid line represents $\rho_{11}$ and the dot line represents $\rho_{22}$, the populations present Rabi oscillations.

Let's consider two comparable coupled subsystems with only one state in each (Fig. 1a). The whole system is described by

$$\mathcal{H}_2 = E_1 a^\dagger a + E_2 b^\dagger b + \Omega(a^\dagger b + b^\dagger a), \tag{3}$$

$a^\dagger$ and $a$ are creation and annihilation operator in subsystem I respectively, $b^\dagger$ and $b$ in subsystem II. Now if we are interested primarily in I, the effect of II through a self-energy is

$$\Sigma_2(\varepsilon) = \frac{\Omega}{\varepsilon - E_1 + i0^+}. \tag{4}$$

However, II is not a reservoir in the common sense. The fundamental feature of a reservoir is that the rate constant for outflow or inflow (e.g., heat flow, current flow) remains unaffected by the filling and vacuuming of states and other dynamical details [1]. II does not satisfy this criterion because the escape rate is

$$\gamma_2 = i(\Sigma_2 - \Sigma_2^\dagger) = \frac{\Omega^2 0^+}{(\varepsilon - E_1)^2 + (0^+)^2} \tag{5}$$

which is affected strongly by $0^+$ (a proper reservoir should be independent of $0^+$). This means that rate out of I is affected by the rate into it. By using the von-Neumann equation $\frac{\mathrm{d}\rho}{\mathrm{d}t} = -i[\mathcal{H}_2, \rho]$ we could calculate the populations $(\rho_{11}, \rho_{22})$ of desity matrix $\rho$ as a function of time. The system is then driven between subsystems, and the populations present Rabi oscillations with frequency $\Omega$, as is shown in Fig. 1c.

Now consider two coupled subsystems with the subsystem II consisting of $N$ states (e.g., a chain with $N$ sites, see Fig. 1b), the resulting Hamiltonian is

$$\mathcal{H}_{\mathrm{N+1}} = E_1 a^\dagger a + E_2 \sum_i b_i^\dagger b_i + \left[ t \sum_i b_i^\dagger b_{i+1} + \Omega a^\dagger b_1 + h.c. \right]. \tag{6}$$

The eigenenergies of II are given by $\varepsilon_n = E_2 + 2t\cos k_n$ and the corresponding normalized wavefunction is $\phi = \sqrt{\frac{2}{N}} \sin k_n x$, where $k_n = n\frac{\pi}{N}, n \in \mathbb{Z}$. So, the effect of II through the self-energy is

$$\Sigma_{\mathrm{N+1}}(\varepsilon) = \frac{2}{N} \sum_n \frac{\Omega^2 \sin^2 k_n}{\varepsilon - \varepsilon_n + i0^+}. \tag{7}$$

When $N \to \infty$, convert the summation to an integral:

$$\Sigma_\infty = \frac{2}{\pi} \int_0^\pi \mathrm{d}k \frac{\Omega^2 \sin^2 k_n}{\varepsilon - \varepsilon_n + i0^+}, \tag{8}$$

and we have $\Sigma_\infty = \Omega e^{ik}$ (we set $E_1 = E_2$ for simplicity). The escape rate is $\gamma_\infty = i(\Sigma_\infty - \Sigma_\infty^\dagger) = 2\Omega \sin k$. By contrast, the reservoir II with $N \to \infty$ states has a constant escape rate independent of $0^+$.

## II. EDGE STATE HAMILTONIAN

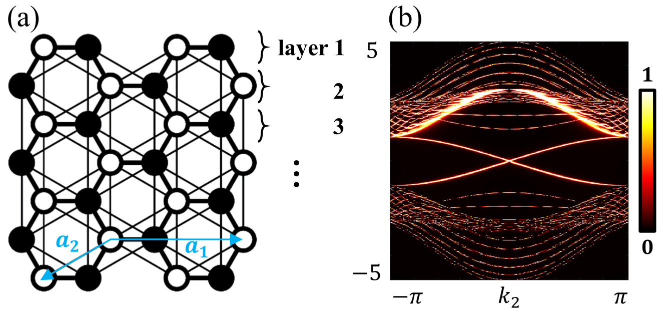


FIG. 2. (a) A semi-infinite two-dimensional honeycomb lattice and a chain of layers. $a_1$ and $a_2$ are the lattice unit vectors. We use the non-orthogonal coordinate based on $a_1$ and $a_2$, and reciprocal space $(k_1, k_2)$ corresponds to that coordinate. (b) Local density of states of $G(\varepsilon; k_1, l)$.

There are several ways to calculate the exact solutions of the edge states, such as via extending Bloch's theorem [2–4], the impurity Green's function [5, 6], the transfer matrix [7, 8], the geometric algebra [9] and so on. The difficulty for the Haldane model roots in the next-nearest neighbor hopping. Here, we follow the approach using the Green's function [9]. The calculation is summarized as follows: we begin with a model $h_0(\mathbf{k})$ with fully periodic boundary conditions, which allows us to write down the Hamiltonian in the momentum space; next, we add hopping perturbation $h_1(k_1)$ that substrate the interaction crossing the first row and the end row of the lattice, forming an open boundary along that direction; the final

Green's function of the resulting system $h_0 + h_1$ is given by the Dyson equation, and the poles of it enable the analytic solution of the edge states. Note that the geometric algebra method can not be applied here since the next-nearest neighbor hopping appears and the supercell Hamiltonian (e.g., two unit cells) is not of Dirac form.

### A. Green's function with periodic boundaries

After Fourier transform, the Haldane model of Eq. 1 in the main text ($t_1 = 1$, Fig. 2a) can be expressed in a compact form as $h_0(\mathbf{k}) = \mathbf{d}\cdot\boldsymbol{\sigma}$, where

$$\begin{aligned} d_x &= 2t_2\left[\sin k_2 + \sin(k_1+k_2) - \sin(k_1+2k_2)\right], \\ d_y &= 1 + \cos k_2 + \cos(k_1+k_2), \\ d_z &= -\sin k_2 + \sin(k_1+k_2). \end{aligned} \tag{9}$$

And the spectrum of the model is $\varepsilon_{\mathbf{k}} = \pm\sqrt{d_x^2 + d_y^2 + d_z^2}$. Correspondingly, the Green function in $\mathbf{k}$ space is

$$G_0(E;\mathbf{k}) = \frac{1}{\varepsilon - h_0(\mathbf{k})} = \frac{1}{\varepsilon^2 - \varepsilon_{\mathbf{k}}^2}\begin{pmatrix} \varepsilon + d_z & d_x - id_y \\ d_x + id_y & \varepsilon - d_z \end{pmatrix} \tag{10}$$

To include the hopping perturbation, we keep the momentum coordinate $k_1$ but perform an inverse Fourier transform to write down the Green's function in real-space coordinate in the $a_2$ direction. Thus, we have

$$G_0(E;k_1,l) = \begin{pmatrix} g_0 & g_1^\dagger & g_2^\dagger & \cdots & g_2 & g_1 \\ g_1 & g_0 & g_1^\dagger & g_2^\dagger & & g_2 \\ g_2 & g_1 & g_0 & g_1^\dagger & & \\ \vdots & g_2 & g_1 & g_0 & & \\ g_2^\dagger & & & & & \\ g_1^\dagger & g_2^\dagger & & & & \ddots \end{pmatrix}_{n,n} \tag{11}$$

where

$$\begin{aligned} g_0 &= \int \frac{\mathrm{d}k_2}{2\pi} G_0(\varepsilon,\mathbf{k}), \\ g_1 &= \int \frac{\mathrm{d}k_2}{2\pi} e^{ik_2} G_0(\varepsilon,\mathbf{k}), \\ g_2 &= \int \frac{\mathrm{d}k_2}{2\pi} e^{2ik_2} G_0(\varepsilon,\mathbf{k}), \end{aligned} \tag{12}$$

and $l = ja_2$ with $j = 1, 2, ..., n$. $G_0(\varepsilon; k_1, l)$ is a $n$-by-$n$ block matrix.

### B. Hopping perturbation

Hopping perturbation $h_1(\varepsilon; k_1, l)$ deletes the hopping crossing the first row and the end row of the lattice, such that it creates two edges perpendicular to $a_1$. Its explicit expression is

$$h_1(\varepsilon;k_1,l) = \begin{pmatrix} 0 & \cdots & v_2 & v_1 \\ \vdots & & 0 & v_2 \\ & & & \\ v_2^\dagger & 0 & \ddots & \\ v_1^\dagger & v_2^\dagger & & 0 \end{pmatrix}_{n,n} \tag{13}$$

where

$$\begin{aligned} v_1 &= \begin{pmatrix} -it_2(1+e^{ik_1}) & 1 \\ e^{ik_1} & it_2(1+e^{ik_1}) \end{pmatrix}, \\ v_2 &= \begin{pmatrix} it_2 e^{ik_1} & 0 \\ 0 & it_2 e^{-ik_1} \end{pmatrix} \end{aligned} \tag{14}$$

$v_1(v_2)$ describes the nearest (next-nearest) neighbor hopping between the layers along $a_2$.

### C. Green's function with the perturbation

The Dyson equation gives the full Green's function $G(\varepsilon; k_1, l)$ in terms of the initial Green's function $G_0(\varepsilon; k_1, l)$ and the hopping perturbation $h_1$, that is

$$G(\varepsilon;k_1,l) = \frac{G_0}{1 - G_0 h_1}. \tag{15}$$

The $G_0$ has no poles in the gap, so the poles of $G$, alternatively the zeros of $\det(1 - G_0 h_1)$, are the edge state eigenvalues when $\varepsilon \in \mathbb{G}$. To show that, we numerically calculate the local density of states given in general by $n(\varepsilon; k_1) = -\frac{1}{\pi}\mathrm{Im}[\mathrm{tr}G(\varepsilon; k_1, l)]$ (see Fig. 2b). Taking the ansatz of edge state wave vector $\phi = \left(u, \lambda u, \lambda^2 u, \ldots, 0\right)^{\mathrm{T}}_{1,n}$ and substituting 11 and 13 into 15, we have

$$(\mathbb{I}-G_0h_1)\,\phi=\begin{pmatrix} I-\begin{pmatrix} g_2 & g_1\\ g_3 & g_2\end{pmatrix}\begin{pmatrix} v_2 & v_1\\ 0 & v_2\end{pmatrix}^\dagger & & -\begin{pmatrix} g_0 & g_1^\dagger\\ g_1 & g_0\end{pmatrix}\begin{pmatrix} v_2 & v_1\\ 0 & v_2\end{pmatrix}\\ & I & \\ \vdots & \ddots & \vdots\\ & & I \\ -\begin{pmatrix} g_0 & g_1^\dagger\\ g_1 & g_0\end{pmatrix}\begin{pmatrix} v_2 & v_1\\ 0 & v_2\end{pmatrix}^\dagger & & I-\begin{pmatrix} g_2 & g_1\\ g_3 & g_2\end{pmatrix}^\dagger\begin{pmatrix} v_2 & v_1\\ 0 & v_2\end{pmatrix}\end{pmatrix}\begin{pmatrix} u\\ \lambda u\\ \\ \vdots\\ \\ 0\end{pmatrix} \tag{16}$$

The ellipses indicate the non-zero subblock. $\phi$ localizes at the first layer and the $|\lambda|<1$ promises the localization. And,

$$\left[I-\begin{pmatrix} g_2 & g_1\\ g_3 & g_2\end{pmatrix}\begin{pmatrix} v_2 & v_1\\ 0 & v_2\end{pmatrix}^\dagger\right]\begin{pmatrix} u\\ \lambda u\end{pmatrix}=0,$$
$$\begin{pmatrix} g_0 & g_1^\dagger\\ g_1 & g_0\end{pmatrix}\begin{pmatrix} v_2 & v_1\\ 0 & v_2\end{pmatrix}^\dagger\begin{pmatrix} u\\ \lambda u\end{pmatrix}=0, \tag{17}$$

which together require (Kramer criterion)

$$\det\begin{pmatrix} g_0 & g_1^\dagger\\ g_1 & g_0\end{pmatrix}=0. \tag{18}$$

It can be further simplified by a decomposition in terms of triangular matrices (note that $\det(g_0)\neq 0$),

$$\det\begin{pmatrix} g_0 & g_1^\dagger\\ g_1 & g_0\end{pmatrix}=\det\left[\begin{pmatrix} g_0 & 0\\ g_1 & I\end{pmatrix}\begin{pmatrix} I & g_0^{-1}g_1^\dagger\\ 0 & g_0-g_1g_0^{-1}g_1^\dagger\end{pmatrix}\right]$$
$$=\det(g_0)\det(g_0-g_1g_0^{-1}g_1^\dagger) \tag{19}$$

So, we can calculate the edge state spectrum explicitly by solving $\det(g_0-g_1g_0^{-1}g_1^\dagger)=0$. The edge states energy is given by $\varepsilon_\pm(k_1)=\pm\sin(k_1/2)$ with $\varepsilon\in\mathbb{G}$, and $+(-)$ corresponds to the state localized at the first (last) layer.

### D. Edge state wave vector

We can also calculate the $u$ through Eq. 17. A more convenient method is by extending Bloch's theorem. In our case, we extend the $k_2$ to the complex domain $\mathbb{C}$ with an analytic continuation, and we have $h_0(k_1,k_2')u=\varepsilon_+(k_1)u$ with $k_2\to k_2'\in\mathbb{C}$. Then the secular equation gives $\det\left[\varepsilon_+-h_0(k_1,k_2')\right]=0$. With $k_2'$, $u$ has the form

$$u=\begin{pmatrix} 1\\ \frac{\varepsilon_+-d_3(k_2')}{d_1(k_2')-id_2(k_2')}\end{pmatrix}, \tag{20}$$

where the argument $k_1$ is suppressed. The normalized solution to this equation is $u=\frac{1}{\sqrt{2}}\left(1,e^{-i\frac{k_1-\pi}{2}}\right)^{\mathrm{T}}$.

Finally, we can use the edge state projector $uu^\dagger$ to construct the effective edge Hamiltonian

$$H_{\text{edge}}=\varepsilon_+uu^\dagger=\frac{1}{2}\begin{pmatrix} \sin\frac{k_1}{2} & \frac{1}{2}(1-\mathrm{e}^{ik_1})\\ \frac{1}{2}(1-\mathrm{e}^{-ik_1}) & \sin\frac{k_1}{2}\end{pmatrix}. \tag{21}$$

Another normalized solution with respect to $\varepsilon_-$, i.e., state locolized at the last layer, is $u'=\frac{1}{\sqrt{2}}\left(1,e^{-i\frac{k_1+\pi}{2}}\right)^{\mathrm{T}}$. Taking two edge states together, the effective Hamiltonian is

$$H'_{\text{eff}}=\varepsilon_+uu^\dagger+\varepsilon_-u'u'^\dagger=\frac{1}{2}\begin{pmatrix} 0 & 1-\mathrm{e}^{ik_1}\\ 1-\mathrm{e}^{-ik_1} & 0\end{pmatrix} \tag{22}$$

It's very interesting that $H'_{\text{eff}}$ is equivalent to the Su-Schrieffer-Heeger model.

## III. SELF-ENERGY

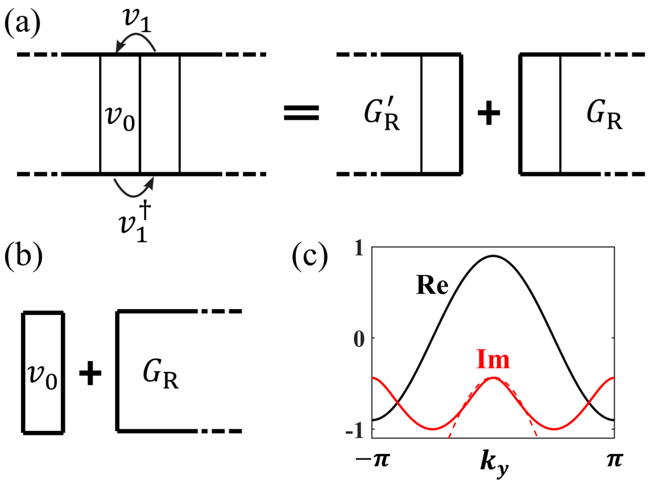


FIG. 3. (a) A full Green's function can be constructed by combining two surface Green's function. (b) The semi-infinite reservoir does not change upon adding another block $v_0$. (c) Self-energy of the square lattice (solid lines). $\lambda_1=1$, $\lambda_2=-0.9$ and $\mu=\varepsilon=0$, hence $\mathrm{Re}(\Sigma)=0.9\cos k_y$ and $\mathrm{Im}(\Sigma)\approx 1.13\cos k_y-1.56$ around $k_y=0$ (dashed line).

The formal expression to evaluate the self-energy is $\Sigma=WG_{\mathrm{R}}W^\dagger$, where $G_{\mathrm{R}}$ represents the surface Green's function and $W$ is the coupling between the closed system and the reservoir. A stable algorithm based on the Schur decomposition (as well as the conventional method using the eigendecomposition) to calculate $G_{\mathrm{R}}$ can be found in Ref. [10]. Here, we follow the procedure using the transfer matrix [11].

Constructing blocks from the reservoir lattice, so that the system is periodic in those blocks $v_0$ and the hopping $v_1$ between them is restricted to the nearest neighbor, as shown in Fig. 3a. In terms of those blocks, we have the recursion relation of subblock matrix of the Green's function

$$g_{\mathrm{n}+1} = v_1^{-1}(\varepsilon - v_0)g_{\mathrm{n}} - v_1^{-1}v_1^{\dagger}g_{\mathrm{n}-1}, \tag{23}$$

which can be rewritten as

$$\begin{pmatrix} g_{\mathrm{n}+1} \\ g_{\mathrm{n}} \end{pmatrix} = \begin{pmatrix} v_1^{-1}(\varepsilon - v_0) & -v_1^{-1}v_1^{\dagger} \\ I & 0 \end{pmatrix} \begin{pmatrix} g_{\mathrm{n}} \\ g_{\mathrm{n}-1} \end{pmatrix} \equiv \mathrm{T} \begin{pmatrix} g_{\mathrm{n}} \\ g_{\mathrm{n}-1} \end{pmatrix}. \tag{24}$$

The above expression requires $v_1$ is nonsingular. If it is singular, refer to Ref. [8]. Then surface Green's function is obtained from

$$G_{\mathrm{R}} = \left[\varepsilon - v_0 - v_1 \mathcal{S}_2 \mathcal{S}_1^{-1}\right]^{-1} \tag{25}$$

or

$$G'_{\mathrm{R}} = \left[\varepsilon - v_0 - v_1^{\dagger} \mathcal{S}_3 \mathcal{S}_4^{-1}\right]^{-1}. \tag{26}$$

$G_{\mathrm{R}}$ or $G'_{\mathrm{R}}$ depends on which semi-infinite part one is interested in (Fig. 3a). $\mathcal{S}_{\mathrm{i}}, \mathrm{i} = 1,2,3,4$ is the subblock of the matrix whose column vectors are ordered eigenvectors of T, i.e.,

$$\begin{pmatrix} \mathcal{S}_2 & \mathcal{S}_4 \\ \mathcal{S}_1 & \mathcal{S}_3 \end{pmatrix}^{-1} \mathrm{T} \begin{pmatrix} \mathcal{S}_2 & \mathcal{S}_4 \\ \mathcal{S}_1 & \mathcal{S}_3 \end{pmatrix} = \begin{pmatrix} \rho_1 & \\ & \ddots \end{pmatrix}. \tag{27}$$

$(\mathcal{S}_2, \mathcal{S}_1)^{\mathrm{T}}$ corresponds to the eigenvalue $\rho_{\mathrm{i}} < 1$ and $(\mathcal{S}_4, \mathcal{S}_3)^{\mathrm{T}}$ corresponds to the eigenvalue $\rho_{\mathrm{i}} > 1$ respectively. In general, they are not independent and are related by a symmetry (e.g., inversion symmetry).

The self-energy $\Sigma$ has a very simple form if one notices the semi-infinite reservoir does not change upon adding another block $v_0$. With $\Sigma$, the Green's function on the additional block is

$$G_{\mathrm{R}} = (\varepsilon - v_0 + \Sigma)^{-1}. \tag{28}$$

Compare with Eq. 25, we have $\Sigma = -v_1 \mathcal{S}_2 \mathcal{S}_1^{-1}$.

For the lattice Hamiltonian $\mathcal{H}_{\mathrm{Cond}}$ in Eq. 2 in the main text, $v_0 = 2\lambda_2 \cos k_y + \mu$, $v_1 = \lambda_1$, so

$$\Sigma = -\frac{1}{2}(\Lambda + \sqrt{-4\lambda_1^2 + \Lambda^2}) \tag{29}$$

with $\Lambda = \mu - \varepsilon + 2\lambda_2 \cos k_y$.

## IV. RESPONSE PROFILE

Here, we give some simple examples to illustrate the response profile, which is an indicator of non-Bloch transport. The model is the Hatano-Nelson model under the open boundary condition:

$$\mathcal{H}_{\mathrm{HN}} = \sum_i \left[te^{i\vartheta} a_i^{\dagger} a_{i+1} + te^{-i\vartheta} a_{i+1}^{\dagger} a_i - i\mu a_i^{\dagger} a_i\right], \tag{30}$$

where we add the global complex onsite potentials $\mu$. Henceforth we set the nearest neighbor hopping $t$ parameter to unity.

- Hermitian case: $\vartheta = \frac{\pi}{2}$ and $\mu = 0$. The response profile corresponding to a excitation is shown in Fig. 4b, and the excited Bloch wave propagates without attenuation.

- NH case with a global dissipation: $\vartheta = \frac{\pi}{2}$ and $\mu = 0.05$, the eigenvalues of $\mathcal{H}_{\mathrm{HN}}$ are in the complex domain owing to $\mu$, but $\mu$ does not lead to NH skin effect. As shown in Fig. 4c, the attenuation shows no inclination to the propagation orientation, thus the response profile corresponding to a excitation is $\propto \begin{cases} e^{\beta y}, & y < 0 \\ e^{-\beta y}, & y > 0 \end{cases}, \beta \in \mathbb{R}$, whcih consists with our intuition of wave attenuation owing to the loss.

- Pseudo-Hermitian case with skin effect: $\vartheta = \frac{\pi}{2} + 0.05i$ and $\mu = 0$, the eigenvalues of $\mathcal{H}_{\mathrm{HN}}$ are all real numbers due to pseudo-Hermiticity $\eta^{-1}\mathcal{H}_{\mathrm{HN}}\eta = \mathcal{H}_{\mathrm{HN}}$. The eigenstates pile up at the boundary, exhibiting NH skin effect. The response profile corresponding to a unit excitation is shown in Fig. 4d, and the profile $\propto e^{\alpha y}, \alpha \in \mathbb{R}$ because of the skin effect.

- NH case with both the skin effect and the global dissipation: $\vartheta = \frac{\pi}{2} + 0.05i$ and $\mu = 0.15$. Figure 4e shows the calculated response profile, which

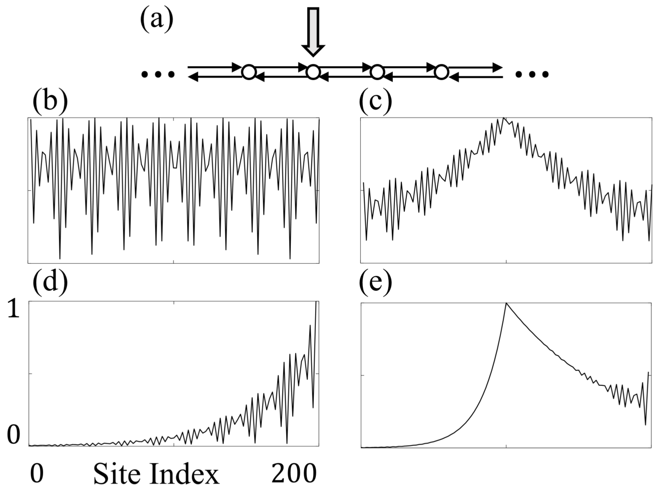


FIG. 4. Response profile corresponding to a unit impulse (Dirac delta function, $E = 0.279$). (a) Hatano-Nelson model. (b) Hermitian case. (c) NH case with global dissipation. (d) Pseudo-Hermitian case. (e) NH case under skin effect and global dissipation.

is roughly $\sim \begin{cases} e^{(\alpha+\beta)y}, & y<0 \\ e^{(\alpha-\beta)y}, & y>0 \end{cases}$. The dacay (or growth) rate is orientation-dependent under the competition between skin effect and global dissipation.

Figure 5 shows some calculated results of the effective chain model (see text around Eq. 5 in the main text).

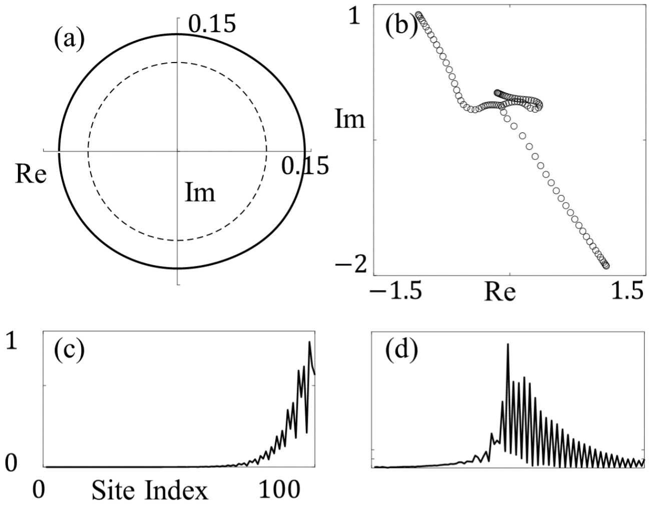


FIG. 5. Calculated results of the effective chain model. (a) Generalized Brillouin zone. In ploting, we use $(|\beta| - 0.99)\, e^{i\mathrm{Arg}(\beta)}$, $\beta = e^{i\tilde{k}}$ in which $\tilde{k}$ is the complex wave number. (b) Eignvalues of the chain Hamiltonian with open boundaries. (c) Eigenvector with respect to the eigenvalue $E = 0$. (d) Response profile corresponding to a unit impulse ($E = 0.028$)

## V. REALIZATION OF THE HOPPING WITH A PHASE

Our previous works [12, 13] develop a correspondence between circuit networks and tight-binding lattice models. We want to apply this theory to higher-frequency regions, such as radio and optical frequencies. Higher frequencies imply decreasing wavelengths. This follows that voltages and currents no longer remain spatially uniform when compared to the geometric size of the discrete circuit elements. As a consequence, they have to be treated as propagating waves. Since Kirchhoff's voltage and current laws do not account for these spatial variations, we must significantly adjust the analysis from conventional lumped to distributed circuit representation.

Multiple port networks are essential tools in restructuring and simplifying complicated circuits as well as in providing key insight into the performance of devices. To describe such network input-output parameter relations, we have impedance, admittance, S-parameter, hybrid, and ABCD parameters–conversions exist between these sets. However, some relations may not be well-defined, such as the admittance of a circulator (see subsection 1), causing difficulty in finding the correspondence between higher-frequency networks and tight-binding lattice models. The principal advances of the S-parameter are that: (i) it is always well-defined in a passive device; (ii) the experimental determination of it is convenient without the need to know the internal structure of the device. Here, we show how to realize the hopping with a phase (we set the coupling amplitude to unity) in the TTC network by designing the S-parameter (see subsection 2-4) when the admittance of the device is not available. The phased-hopping breaks the reciprocity, i.e., $t_{ij} \neq t_{ji}$, so we use a circulator to realize this hopping. The 'black box' treatment of the S-parameter indicates that distinct devices or different network configurations can realize the same phased-hopping since they may have an identical S-parameter (see subsection 4). The calculation of S-parameters is based on the signal flow graph, subsection 2 will provide some context.

### A. Ill-defined admittance of microwave circulators

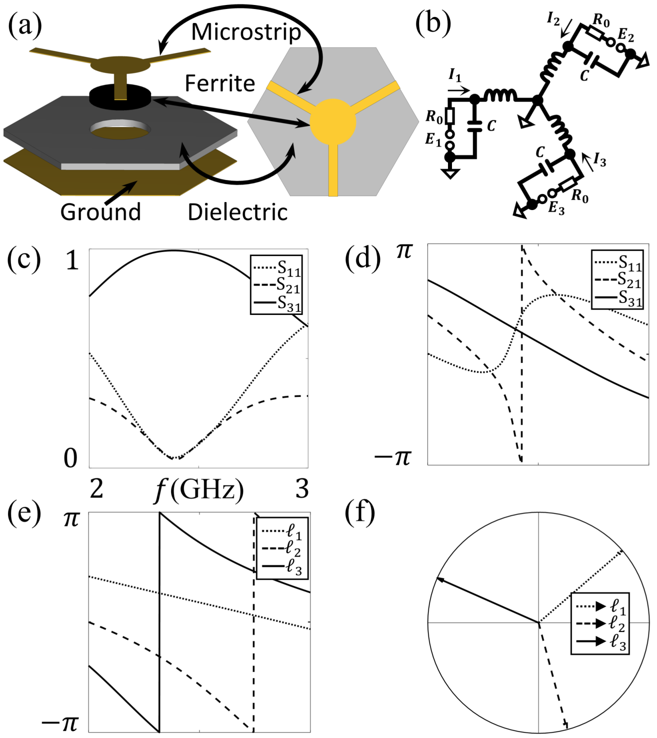


FIG. 6. (a) Schematic of a three-port microstrip circulator. (b) Shunt network of lumped element circulator. (c) and (d) Scattering parameters (amplitude and phase) of the circulator from CST simulation. (e) Characteristics $(\ell_1, \ell_2, \ell_3)$ as function as the frequency varies, the circulator resonates at 2.4 GHz. (f) Eigenvalues of the scattering matrix at 2.4 GHz, $\mathrm{u}^{-1} S \mathrm{u} = \mathrm{diag}(e^{i\ell_1}, e^{i\ell_2}, e^{i\ell_3})$, where $(\ell_1, \ell_2, \ell_3) = \left(\ell_0, \ell_0 + \frac{2\pi}{3}, \ell_0 - \frac{2\pi}{3}\right)$ and $\ell_0 \approx 0.71$.

The circulator geometry (Fig. 6a) can readily be analyzed using the lumped element configuration (Fig. 6b illustrates the network). The usual arrangement consists of a ferrite disk with three strips wound on it: i) the strips are oriented at 120° with respect to each other and are electrically short at the end of them; ii) a direct magnetic field $H_0$ is applied normal to the plane of the circulator, so the relative permeability tensor $\mu_{ij}$ of the ferrite disk is

$$[\mu_{ij}] = \begin{pmatrix} \mu & -i\kappa & 0 \\ i\kappa & \mu & 0 \\ 0 & 0 & 1 \end{pmatrix}. \tag{31}$$

with

$$\mu = 1 + \frac{\omega_0\omega_m}{\omega_0^2 - \omega^2}, \qquad \kappa = \frac{\omega\omega_m}{\omega^2 - \omega_0^2}. \tag{32}$$

$\omega_0 = \gamma(H_0 - N_z M_s)$, and $\omega_m = \gamma M_s$, where $M_s$ is the saturation magnetization, $\gamma$ is the gyromagnetic ratio, $N_z$ is the demagnetizing factor. The presence of imaginary off-diagonal components having opposite signs in $\mu_{ij}$ is the basis for the nonreciprocal effect.

The energy within the disk is essentially magnetic because of shorted strips. That follows that the simplified equivalent circuit in the disk, which retains all of the electrical characteristics, contains three mutual inductances. Shunt capacities out of the disk are added to maintain the characteristic impedance. So, the voltage–current relationships (impedance) at the terminals of the disk structure are

$$\begin{pmatrix} V_1 \\ V_2 \\ V_3 \end{pmatrix} = i\omega L_0 \begin{pmatrix} \mu & \frac{i\kappa-\mu}{2} & \frac{-i\kappa-\mu}{2} \\ \frac{-i\kappa-\mu}{2} & \mu & \frac{i\kappa-\mu}{2} \\ \frac{i\kappa-\mu}{2} & \frac{-i\kappa-\mu}{2} & \mu \end{pmatrix} \begin{pmatrix} I_1 \\ I_2 \\ I_3 \end{pmatrix} \equiv Z \begin{pmatrix} I_1 \\ I_2 \\ I_3 \end{pmatrix}. \tag{33}$$

Note that $Z \neq Z^{\mathrm{T}}$ as $\mu_{ij} \neq \mu_{ji}$.

The admittance of the circulator, which is the inverse of $Z$, is ill-defined since its impedance $Z$ is singular (i.e., the voltages do not determine the currents). Nevertheless, we can calculate the pseudoinverse of $Z$,

$$Z^{+} = \frac{4\mu}{3(-\kappa^2 + 3\mu^2)} \frac{1}{i\omega L_0} \begin{pmatrix} \mu & \frac{-i\kappa-\mu}{2} & \frac{i\kappa-\mu}{2} \\ \frac{i\kappa-\mu}{2} & \mu & \frac{-i\kappa-\mu}{2} \\ \frac{-i\kappa-\mu}{2} & \frac{i\kappa-\mu}{2} & \mu \end{pmatrix}. \tag{34}$$

One can hardly find any correspondence to $\mathcal{H}_\Delta$.

The scattering matrix $S$ however is well-defined (note that every passive circuit has a scattering matrix [14]), and $SS^\dagger = 1$ if the network is dissipationless. The circulator respects C3 symmetry, thus we can use the frame u defined in the main text to diagonalize the matrix, $\mathrm{u}^{-1}S\mathrm{u} = \mathrm{diag}(e^{i\ell_1}, e^{i\ell_2}, e^{i\ell_3})$. This also follows that $S_{11} = S_{22} = S_{33}$, $S_{12} = S_{23} = S_{31}$ and $S_{21} = S_{32} = S_{13}$. Similarly, the eigenvalues uniquely define the scattering relation between ports.

Figure 6c and d show the scattering parameters of the circulator and its characteristics as frequency varies. At the resonant frequency of the circulator, the scattering matrix is approximate to an ideal circulator:

$$S_{\mathrm{id}} = e^{i\ell_0} \begin{pmatrix} 0 & 0 & 1 \\ 1 & 0 & 0 \\ 0 & 1 & 0 \end{pmatrix}, \tag{35}$$

and the characteristics are $(\ell_1, \ell_2, \ell_3) = \left(\ell_0, \ell_0 + \frac{2\pi}{3}, \ell_0 - \frac{2\pi}{3}\right)$.

## B. Review of signal flow graphs

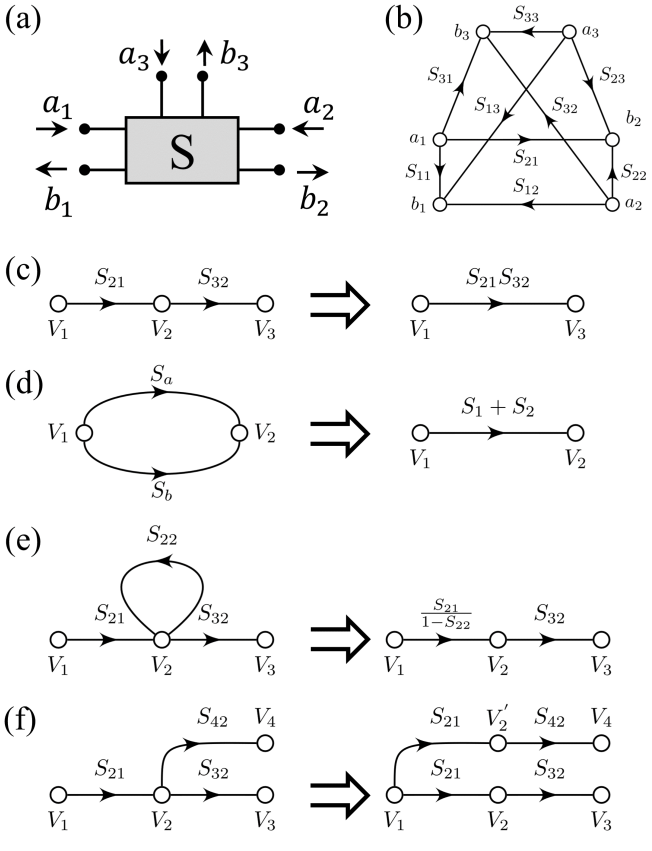


FIG. 7. The signal flow graph representation of a three-port network and decomposition rules of flow graph. (a) A general three-port network and (b) its signal flow graph. Decomposition rules: (c) Series rule, (d) Parallel rule, (e) Self-loop rule, (f) Splitting rule.

The analysis of networks is greatly facilitated through signal flow graphs. The primary components of the graph are nodes and branches. Each port $i$ of a network has two nodes: node $a_i$ is deployed to indentify a entering wave, while $b_i$ a reflected wave. A branch is a directed path between two nodes representing signal flow from one node to another. The S-parameter (the scattering

matrix, e.g., Fig. 7a and b) is defined as

$$S_{ii} = \frac{b_i}{a_i}\bigg|_{a_{j\neq i}=0},$$
$$S_{ji} = \frac{b_j}{a_i}\bigg|_{a_{l\neq i}=0}. \quad (36)$$

In the network, we use the normalized incident power wave $a_i$ and reflected power wave $b_i$:

$$a_i = \frac{1}{2\sqrt{Z_0}}(V_n + Z_0 I_n),$$
$$b_i = \frac{1}{2\sqrt{Z_0}}(V_n - Z_0 I_n), \quad (37)$$

where the $Z_0$ is the characteristic impedance of the connecting waveguide on the input and output side of the network. In what follows, we set $Z_0 = 1$ for simplicity. A signal flow graph can be reduced to a single branch between two nodes using the four basic decomposition rules to obtain any desired wave amplitude ratio (Fig. 7c-f).

## C. Two sites

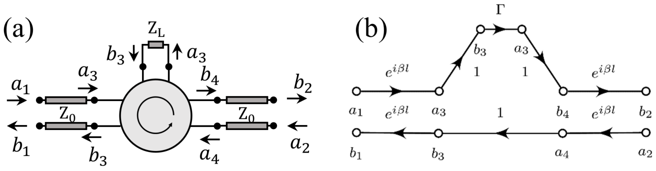


FIG. 8. Realization of two-site hopping with a phase. (a) Schematic of the realization. (b) Corresponding flow graph.

We employ a three-port ideal circulator (we set $\ell_0 = 0$ in Eq. 35 ) to realize the two-site coupling with an arbitrary phase $\theta$ and set the coupling amplitude to unity. The Hamiltonian of the two sites reads

$$\mathcal{H}_2 = \begin{pmatrix} & e^{i\theta} \\ e^{-i\theta} & \end{pmatrix}. \quad (38)$$

The bilinear transform $\frac{i+\mathcal{H}_2}{i-\mathcal{H}_2}$ gives $\begin{pmatrix} & e^{i(\theta-\frac{\pi}{2})} \\ e^{i(\frac{\pi}{2}-\theta)} & \end{pmatrix}$. One can not find a $\theta$-independent frame that diagonalizes the transformed matrix, but we can define two characteristics $\chi_\pm$ as $\chi_\pm = \pm(\theta - \frac{\pi}{2})$ by noting the off-diagonal form of the transformed matrix.

Two ports of the circulator are attached to the waveguides with electrical length $\beta l$, where $\beta$ is the wavenumber in the waveguide and $l$ is the physical length of the waveguide, and the rest port is terminated in a load impedance $Z_L$. Using the flow graph Fig. 8b, the S-parameter of this configuration is

$$S_2 = \begin{pmatrix} & e^{2i\beta l} \\ \Gamma e^{2i\beta l} & \end{pmatrix}, \quad (39)$$

where $\Gamma = \frac{Z_L - Z_0}{Z_L + Z_0}$ is the reflection coefficient. Unitary matrix $S_2 S_2^\dagger = 1$ leads to $|\Gamma| = 1$. Similarly, we can define the characteristics of $S_2$ as is $\ell_+ = 2\beta l$ and $\ell_- = \mathrm{Arg}(\Gamma) + 2\beta l$. $\chi_\pm$ and $\ell_\pm$ give us the correspondence, for example, when $\theta = \frac{\pi}{2}$, $\beta l = 0$, $Z_L = 0$. Note that the load $Z_L$ can be realized by a piece of waveguide with its end grounded or open (see Fig. 12 and text around there).

## D. Three sites

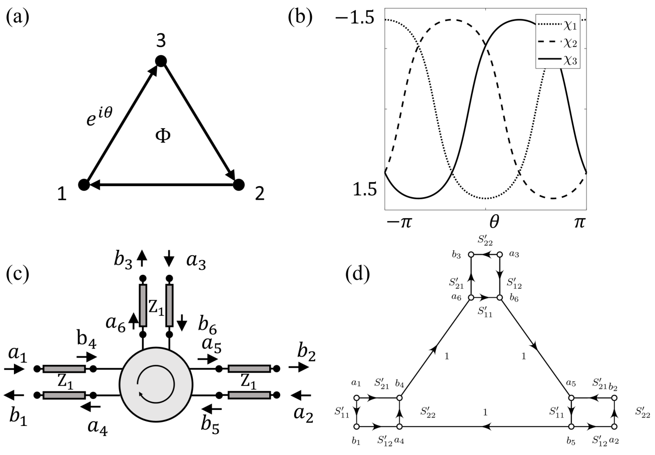


FIG. 9. Realization of three-site hopping with phases. (a) Three-site model with pumped flux Φ. (b) Three characteristics as a function of $\theta$. (c) Schematic of the realization and (d) the corresponding flow graph.

Here, we show how to realize the next-nearest neighbor hopping required in the Haldane model. To illustrate it, consider the following three-site Hamiltonian (Fig. 9a):

$$\mathcal{H}_\Delta = \begin{pmatrix} 0 & e^{i\theta} & e^{-i\theta} \\ e^{-i\theta} & 0 & e^{i\theta} \\ e^{i\theta} & e^{-i\theta} & 0 \end{pmatrix}. \quad (40)$$

The transformed matrix $\mathcal{S} = \frac{i+\mathcal{H}_\Delta}{i-\mathcal{H}_\Delta}$ can be diagonalized by the frame u because of the C3h symmetry: $\mathrm{u}^{-1}\mathcal{S}\mathrm{u} = \mathrm{diag}(e^{i\chi_1}, e^{i\chi_2}, e^{i\chi_3})$, where $\mathrm{u} = (\mathbf{v}_1, \mathbf{v}_2, \mathbf{v}_3)$, $\mathbf{v}_1 = (1,1,1)^{\mathrm{T}}, \mathbf{v}_2 = (1,\alpha,\alpha^2)^{\mathrm{T}}, \mathbf{v}_3 = (1,\alpha^2,\alpha)^{\mathrm{T}}$ with $\alpha = e^{\frac{2\pi i}{3}}$. The characteristics are shown in Fig. 9b as $\theta$ varies.

To realize that, we employ a three-port circulator with its ports attached to waveguides, see Fig. 9c. The waveguides attached have the characteristic impedance of $Z_1$, and the electrical length is $\beta_1 l_1$. Using the flow graph

Fig. 9d, the S-parameter of this configuration is

$$S_{11} = \frac{a(a^3 - ab^2 - 1)}{a^3 - 1}$$
$$S_{12} = \frac{-ab^2}{a^3 - 1}$$
$$S_{21} = \frac{-b^2}{a^3 - 1}, \quad (41)$$

and $S_{11} = S_{22} = S_{33}$, $S_{12} = S_{23} = S_{31}$ and $S_{21} = S_{32} = S_{13}$ due to C3 symmetry of the configuration (i.e. $S$ is a cicular matrix denoted as $S = \mathrm{circ}(S_{11}, S_{12}, S_{13})$). $S' = \begin{pmatrix} a & b \\ b & a \end{pmatrix}$ is the scattering matrix because of the impedance mismatch between connecting waveguides of $Z_0$ and attached waveguides of $Z_1$, $a = e^{i\beta_1 l_1} \frac{Z_0 - Z_1}{Z_0 + Z_1}$. The mirror symmetry of the impedance-mismatch scattering leads to $S'_{12} = S'_{21}$ and $a^2 + b^2 = 1$ follows from $S'S'^{\dagger} = 1$. The characteristics of S-parameter $\ell_{1,2,3}$ (i.e., the eigenvalues of the S-parameter) and characteristics of transformed-matrix $\chi_{1,2,3}$ give the correspondence, for example, when $\theta = \frac{\pi}{2}$, $\beta_1 l_1 = 0$, $Z_1 = Z_0$.

What is unique to the three-port ideal circulator is that we can calculate its admittance through $Y_{\mathrm{id}} = \frac{1 - S_{\mathrm{id}}}{1 + S_{\mathrm{id}}}$ (set $\ell_0 = 0$). An alternative approach to calculating this diagram structure (Fig. 9a) using the Kirchhoff's law can be found around Eq. 58.

### E. Four sites

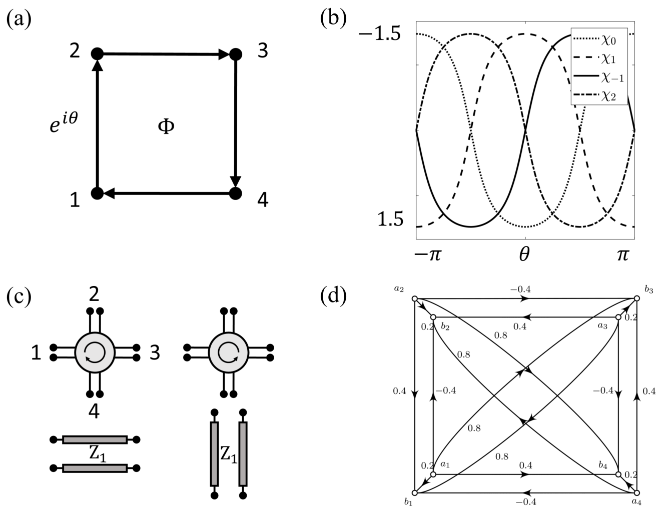


FIG. 10. Realization of four-site hopping with phases. (a) Four-site model with pumped flux Φ. (b) Four characteristics as a function of θ. (c) Schematic of the realization by the channel decomposition and (d) the corresponding flow graph.

Here, we show how to introduce the flux through a four-site plaquette. Without losing generality, we set the coupling amplitude to be unity and the onsite potential to be zero (Fig. 10a). The resulting Hamiltonian is

$$\mathcal{H}_{\Box} = \begin{pmatrix} 0 & e^{i\theta} & 0 & e^{-i\theta} \\ e^{-i\theta} & 0 & e^{i\theta} & 0 \\ 0 & e^{-i\theta} & 0 & e^{i\theta} \\ e^{i\theta} & 0 & e^{-i\theta} & 0 \end{pmatrix}. \quad (42)$$

When $\Phi = 0$, the model respects D4h symmetry, So according to group theory, we can generate the equivalence representation (i.e., transform between equivalent sites) for the symmetry. In this case, the equivalence representation $\Gamma$ is reducible:

$$\Gamma = A_1 \oplus B_1 \oplus E \quad (43)$$

where $A_1$, $B_1$ and $E$ denote the unreducible representation of D4h. $E$ is a 2-by-2 matrix, meaning that two of the four eigenvalues of $\mathcal{H}_{\Box}$ are degenerate. Those two-fold eigenvalues can be lifted by pumping flux $\Phi$, and $\mathcal{H}_{\Box}$ respects C4 symmetry when pumping. So we can use a symmetrical set of basis

$$\mathrm{u} = \begin{pmatrix} 1 & 1 & 1 & 1 \\ 1 & -1 & i & -i \\ 1 & 1 & -1 & -1 \\ 1 & -1 & -i & i \end{pmatrix}. \quad (44)$$

Under this frame $u$, the transformed matrix $\mathcal{S} = \frac{i + \mathcal{H}_{\Box}}{i - \mathcal{H}_{\Box}}$ can be diagonalized as $\mathrm{u}^{-1}\mathcal{S}\mathrm{u} = \mathrm{diag}(e^{i\chi_0}, e^{i\chi_1}, e^{i\chi_{-1}}, e^{i\chi_2})$. Those characteristics are shown in Fig. 10b as $\theta$ varies.

One of the simplest ways to realize $\mathcal{H}_{\Box}$ is by taking advantage of two-site couping (see text around Eq. 38). Here, we introduce the other two ways. Without losing generality, we set $\theta = \frac{\pi}{2}$ in the following.

*I*—If the S-parameter shares the same characteristics as $\mathcal{S}$, $S$ will take the form $S = \mathrm{u} \cdot \mathrm{diag}(e^{i\chi_0}, e^{i\chi_1}, e^{i\chi_{-1}}, e^{i\chi_2}) \cdot \mathrm{u}^{-1}$. $S = \mathrm{circ}(0.2, -0.4, 0.8, 0.4)$ when $\theta = \frac{\pi}{2}$. We can decompose $S$ into several channels, $S = S_{\circlearrowleft} + S_{\circlearrowright} + S_{\nearrow} + S_{\swarrow}$ where $S_{\circlearrowright} = -0.4 \cdot \mathrm{circ}(0, 1, 0, 0)$, $S_{\circlearrowleft} = 0.4 \cdot \mathrm{circ}(0, 0, 0, 1)$,

$$S_{\nearrow} = \begin{pmatrix} 0.2 & 0.8 & & \\ & & & \\ 0.8 & 0.2 & & \\ & & & \end{pmatrix} \text{ and } S_{\swarrow} = \begin{pmatrix} & & & \\ & 0.2 & & 0.8 \\ & & & \\ & 0.8 & & 0.2 \end{pmatrix}. \quad (45)$$

By inspection, we find that $S_{\circlearrowright}$ and $S_{\circlearrowleft}$ are nothing but the S-parameters of four-port right-hand and left-hand circulators. $S_{\nearrow}$ or $S_{\swarrow}$ corresponds to the reciprocal scattering between port-1 and port-3 or scattering between port-2 and port-4 (Fig. 10c). This construction can be easily verified by the sigal flow graph shown in Fig. 10d.

*II*— The above realization is still cumbersome for experiments. The construction discussed here is based on the ferrite eigenvalue adjustment for the 4-port nonreciprocal devices [15–17]. The geometry of a dielectric disk is shown in Fig. 11a. Here, we focus on the resonant modes $\mathrm{HE}_{\pm 1,1,1}$ supported by the disk. Without the external magnetic field, two modes are degenerate due to

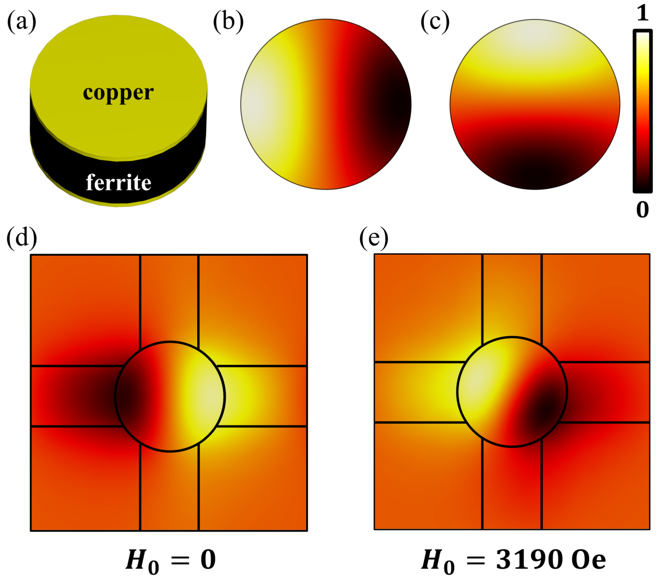


FIG. 11. Realization of Four-site hopping by the ferrite eigenvalue adjustment. (a) Geometry of a dielectric disk. (b) and (c) Field patterns of $\mathrm{HE}_{\pm1,1,1}$. (d) Scattering field distribution without external magnetic field. (e) Scattering field distribution under external magnetic field. Parameters of the ferrite are $\varepsilon_{\mathrm{f}} = 25$, $4\pi M_s = 1800$ Gauss, $\Delta H = 18$ Oe, and the radius of the disk is 2 mm.

the cylinder symmetry of the disk, and their field patterns resemble the $p_x$ and $p_y$ orbitals of an atom (Fig. 11b and c). If we attach four ports to this disk under the C4 symmetry, the S-parameter between ports around the $\mathrm{HE}_{\pm1,1,1}$ eigenfrequency is $S = \mathrm{circ}(0, 0, 1, 0)$. This follows that the excitation from one port only excites one mode of $\mathrm{HE}_{\pm1,1,1}$. For example, excitation from port 1 can only excite $\mathrm{HE}_{1,1,1}$ mode, so it only couples to port 3, and there is no cross-over between channel $1 \leftrightarrow 3$ and channel $2 \leftrightarrow 4$ (Fig. 11d).

Correspondingly, the characteristics of $\mathrm{circ}(0, 0, 1, 0)$ are $(\ell_0, \ell_1, \ell_{-1}, \ell_2) = (0, \pi, \pi, 0)$, $\ell_+ = \ell_-$ because of the D4h symmetry, $\ell_1 = \ell_2$ because of the accidental degeneracy. Those characteristics can be adjusted by the amplitude of the direct magnetic field. This adjustment rotates the standing wave formed by $\mathrm{HE}_{1,1,1}$ to make sure $\ell_{\pm1} = \pm0.7048\pi$ (Fig. 11e), and it lifts the degeneracy of $\ell_1$ and $\ell_{-1}$ without affecting $\ell_0$ and $\ell_2$.

## VI. SIMULATIONS OF MICROSTRIP LINE METAMATERIALS

This section gives the details about simulations of the metamaterials. Firstly, we use microstrip line (ML) to demonstrate the flexibility of TTCs to upgrade to higher frequencies. The ML circuit also exhibits the property of momentum resolution, which is the advantage of TTCs and is demonstrated through ML honrycomb lattice model. Then, the admittance properties of a circulator are analyzed in order to construct Haldane model with ML. Moreover, details about the microwave field-circuit co-simulation of the ML junction are given.

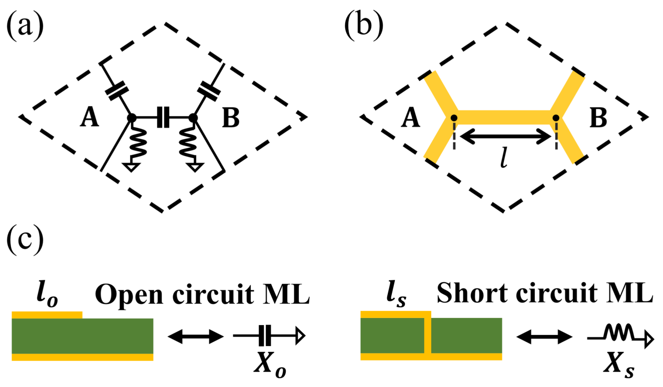


FIG. 12. (a) Unit cell of the circuit honeycomb lattice. (b) Unit cell of ML honeycomb lattice. (c) The equivalent circuit of a red triangle part in (b). (d) The equivalent circuits of open and short ciurcuit ML.

### A. Upgrade of TTCs

To construct the topological junction, we first consider the honeycomb lattice with only the nearest neighbor hopping $t_1$ and onsite potential $\mu$, which is the basis of Haldane model. The Hamiltonian of such lattice reads

$$\mathcal{H}_{\mathrm{Gra}} = t_1 \sum_{\langle i,j \rangle} c_i^\dagger c_j + \mu \sum_i c_i^\dagger c_i \tag{46}$$

and can be realized with temporal topolectrical circuits (TTCs). The unit cell of the corresponding circuit lattice is shown in Fig. 12a. The distance between the sublattices A and B is set to be 1. Thus, the lattice constant is $\sqrt{3}$ and the admittance matrix $J_{\mathrm{Gra}}$ in momentum space reads

$$J_{\mathrm{Gra}} = -i\omega C_1 \begin{pmatrix} 0 & J_{12} \\ J_{12}^\dagger & 0 \end{pmatrix} + (3i\omega C_1 + \frac{1}{i\omega L_1})\mathbb{I}_2$$
$$J_{12} = 1 + \mathrm{e}^{\frac{i}{2}(\sqrt{3}k_x + 3k_y)} + \mathrm{e}^{\frac{i}{2}(-\sqrt{3}k_x + 3k_y)}, \tag{47}$$

where $\omega$ is the operating angular frequency and $\mathbb{I}_n$ is the n-by-n identity matrix. Generally, the nearest neighbor hopping $t_1$ is realized with the capacitor $C_1$ and the onsite potential is adjusted through the grounded inductor $L_1$.

As stated in the main text, TTCs can be upgraded to the microwave domain. Such upgrade is practical for many platforms, e.g., waveguide, coaxial line, ML and so on, and we use ML to illustrate the procedure. ML consists of a dielectric substrate with a conductor strip attached to its surface and the ground plane on the other. Under a certain parameter range, the electromagnetic properties of an ML with width $w$ and length $l$ are equivalent to a Π-shaped circuit as shown in Fig. 4a and 4b in

the main text. The admittances of the components are

$$X_1 = -i\frac{1}{Z_0 \sin k_0 l},$$
$$X_2 = i\frac{1}{Z_0}\tan\frac{k_0 l}{2}, \quad (48)$$

where $Z_0$ is the characteristic impedance and $k_0 = 2\pi/\lambda_0$ is the wave number. The ML parameters are $w = 2.2$ mm, $l = 16.3$ mm, $h = 1.2$ mm, $\varepsilon_r = 4.6$, and $f = 2.4$ GHz, which lead to the impedance $Z_0 = 50\,\Omega$ and the electrical length $k_0 l = \pi/2$. Thus, $X_1 + X_2 = 0$, the self-admittance of both sublattice A and B is equal to 0.

Because of the equivalence, the circuit cell of Fig. 12a can be replaced by ML as shown in Fig. 12b. We construct the ML honeycomb lattice in CST (Fig. 13a) and simulate the field distribution. A waveguide port is set at P and the field within the green box is simulated at $f = 2.4$ GHz. All boundaries are set as perfect electric conductors.

After Fourier Transform (FT), the energy band section at certain momentum is achieved (Fig. 13b). The theoretical result calculated from Eq. 46 is also given for comparison. As an upgrade of TTCs, the ML lattice also exhibits the property of momentum resolution. The momentum at which the band section is obtained after FT can be adjusted by attaching a length of open or short circuit ML to sublattice sites. As shown in Fig. 12c, a length of open (short) circuit ML is equivalent to a grounded capacitor (inductor), whose admittance is

$$X_o = i\frac{1}{Z_0}\tan k_0 l_o,$$
$$X_s = -i\frac{1}{Z_0 \tan k_0 l_s}. \quad (49)$$

Therefore, attaching a length of ML to a site simply alters the self-admittance of it, changing the onsite potential $\mu$. To demonstrate that, simulation at different onsite potentials is caused (Fig. 13c and 13d).

## B. ML Haldane model

To make honeycomb lattice topological, imaginary next-nearest neighbor hopping related with direction is added to break the time-reversal symmetry, which is the Haldane model. For ML lattice, such hopping can be introduced through a circulator (Fig. 14a). The propagation of wave in a circulator depends on the location of the three ports. For an ideal circulator, the S matrix is

$$S_{\mathrm{cir}} = \begin{pmatrix} 0 & 0 & 1 \\ 1 & 0 & 0 \\ 0 & 1 & 0 \end{pmatrix} \quad (50)$$

and the corresponding admittance matrix is

$$J_{\mathrm{cir}} = \frac{1}{Z_0}\begin{pmatrix} 0 & 1 & -1 \\ -1 & 0 & 1 \\ 1 & -1 & 0 \end{pmatrix} = i\frac{1}{Z_0}\begin{pmatrix} 0 & -i & i \\ i & 0 & -i \\ -i & i & 0 \end{pmatrix}. \quad (51)$$

However, an actual circulator always carries a phase shift of $\theta$ and the corresponding S and admittance matrices are

$$S_{\mathrm{act}} = \begin{pmatrix} 0 & 0 & \mathrm{e}^{i\theta} \\ \mathrm{e}^{i\theta} & 0 & 0 \\ 0 & \mathrm{e}^{i\theta} & 0 \end{pmatrix}, J_{\mathrm{act}} = \frac{\mathbb{I}_3 - S_{\mathrm{act}}}{Z_0(\mathbb{I}_3 + S_{\mathrm{act}})}. \quad (52)$$

Moreover, connecting circulators to the lattice sites also requires certain lengths of ML. To calculate the overall admittance $J^{'}_{\mathrm{cir}}$ introduced by an actual circulator, the schematic is shown as Fig. 14b. $I$ and $V$ are the current and voltage respectively, and $l^{'}$ is the length of the connecting ML. The corresponding admittance $X^{'}_1$ and $X^{'}_2$ can be calculated as Eq. 48. Denoting $I = [I_1\ I_2\ I_3]^T$ and the same for $V$, $I^{'}$, and $V^{'}$, then

$$I^{'} = X^{'}_1 V^{'} + X^{'}_2(V^{'} - V), \quad (53)$$

$$X^{'}_2(V^{'} - V) = X^{'}_1 V + I. \quad (54)$$

Noting that $I = J_{\mathrm{act}}V$,

$$I^{'} = X^{'}_1 V^{'} + X^{'}_1 V + J^{'}_{\mathrm{cir}}V, \quad (55)$$

and Eq. 54 can be transformed into

$$V = (\frac{X^{'}_1\mathbb{I}_3 + J_{\mathrm{act}}}{X^{'}_2} + \mathbb{I}_3)^{-1}V^{'}. \quad (56)$$

Substituting Eq. 56 into Eq. 55,

$$I^{'} = (X^{'}_1 + \frac{X^{'}_1\mathbb{I}_3 + J_{\mathrm{act}}}{\frac{X^{'}_1\mathbb{I}_3 + J_{\mathrm{act}}}{X^{'}_2} + \mathbb{I}_3})V^{'}, \quad (57)$$

namely

$$J^{'}_{\mathrm{cir}} = X^{'}_1 + \frac{X^{'}_1\mathbb{I}_3 + J_{\mathrm{act}}}{\frac{X^{'}_1\mathbb{I}_3 + J_{\mathrm{act}}}{X^{'}_2} + \mathbb{I}_3}. \quad (58)$$

Introducing the imaginary next-nearest neighbor hopping to the ML honeycomb lattice with circulators, the ML Haldane lattice with armchair boundaries is constructed as shown in Fig. 15a. The ML Haldane lattice consists of 2 layers (only shown in the inset without substrates and ground plane for clarity): three non-adjacent sites are connected to a ferrite circulator on the top layer, and the other three are connected to another circulator on the bottom layer through vias. The two layers are separated by copper, which serves as the ground plane. Figure 15b shows the corresponding field distribution at $f = 2.4$ GHz, which demonstrates the existence of boundary state. It should be noted that, in simulations, we use ML ferrite circulators as Fig. 6a, while for experimental realization, commercial circulators as Fig. 14a can be used directly to simplify the structure.

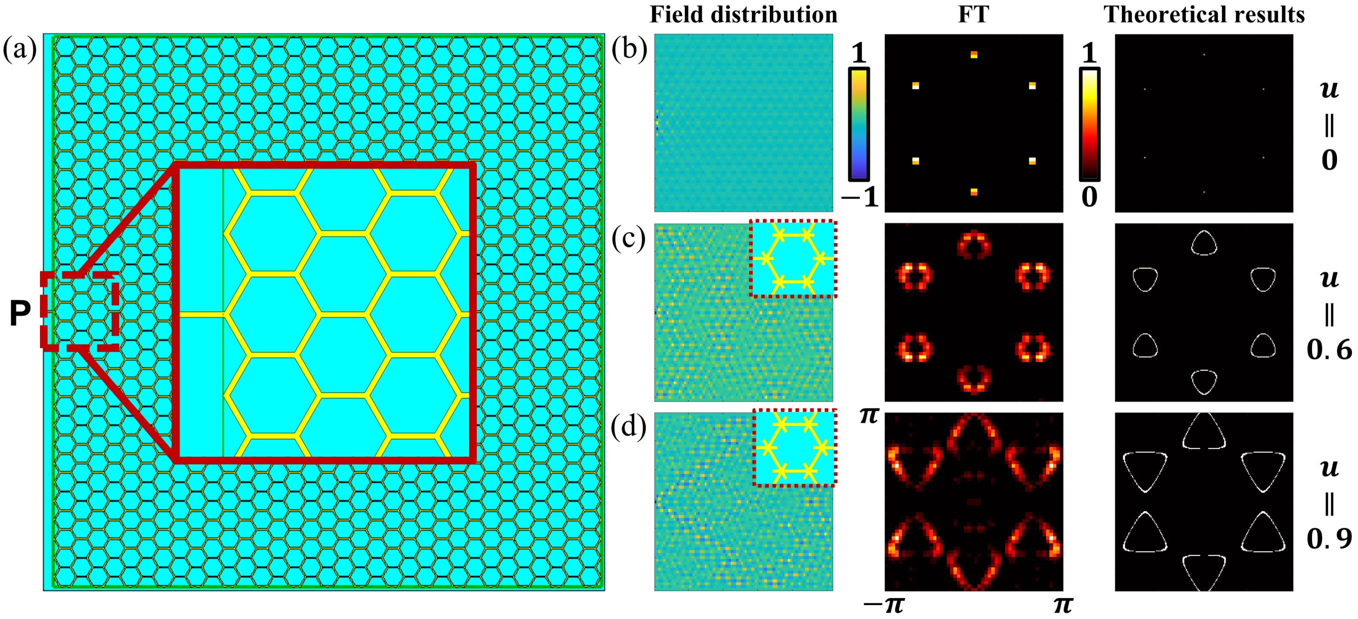


FIG. 13. (a) Simulation model of ML honeycomb lattice. (b)-(d) Simulated field distributions and the corresponding energy band sections at different onsite potentials. Theoretical results are given for comparison.

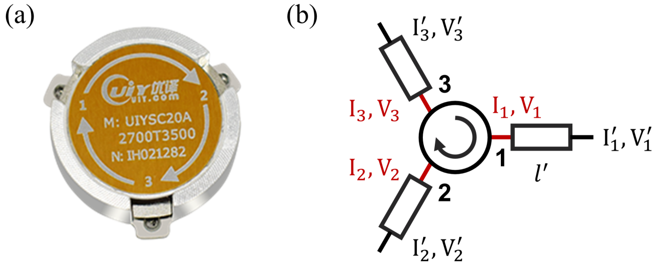


FIG. 14. (a) A circulator. (b) Schematic of connecting a circulator to ML lattice with three lengths of ML.

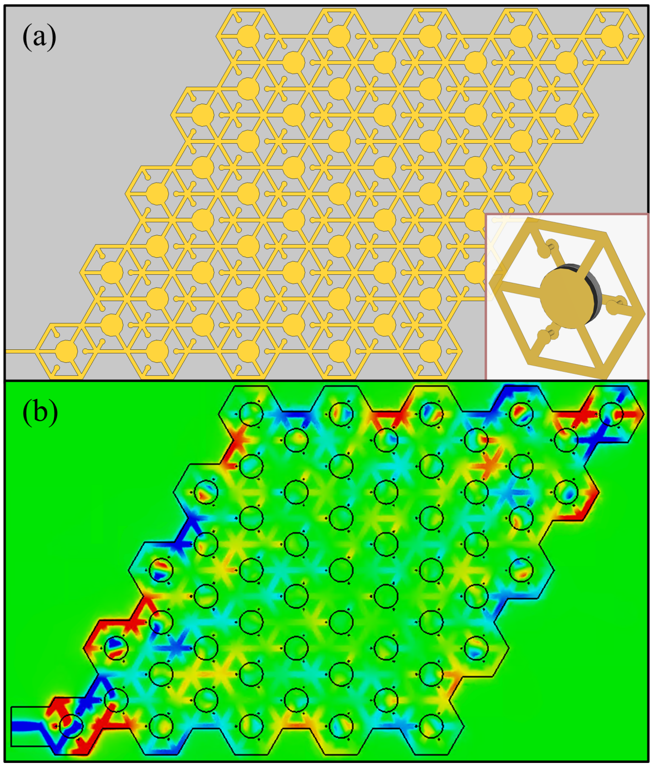


FIG. 15. (a) The simulation model of ML Haldane lattice. (b) Field distribution at $f = 2.4$ GHz.

### C. Field-circuit co-simulation of the junction

Connecting conductors at the boundary of the ML Haldane model can construct the junction. However, due to the large scale and complex multi-layer and thin-layer structures of the junction, simulating a complete model requires extremely high-density meshing and massive computational resources. In addition, we only care about the propagation characteristics of electromagnetic wave within the junction regions rather than the field distributions of the entire model. Thus, we adopt the CST microwave field-circuit co-simulation method to simplify computation and solve the transmission behavior.

Specifically, the model is roughly divided into four parts as shown in Fig. 16:

The component shown in Fig. 16a contains two sublattice sites A and B of the honeycomb lattice. The area indicated by red solid lines (namely, port 1, 3, 6, 8) represents the connection between adjacent sites, while the other ports are used to connect the sites with circulators. Key simulation parameters are ML width $w = 2.2$ mm, distance between adjacent sites $l_{\mathrm{AB}} =$

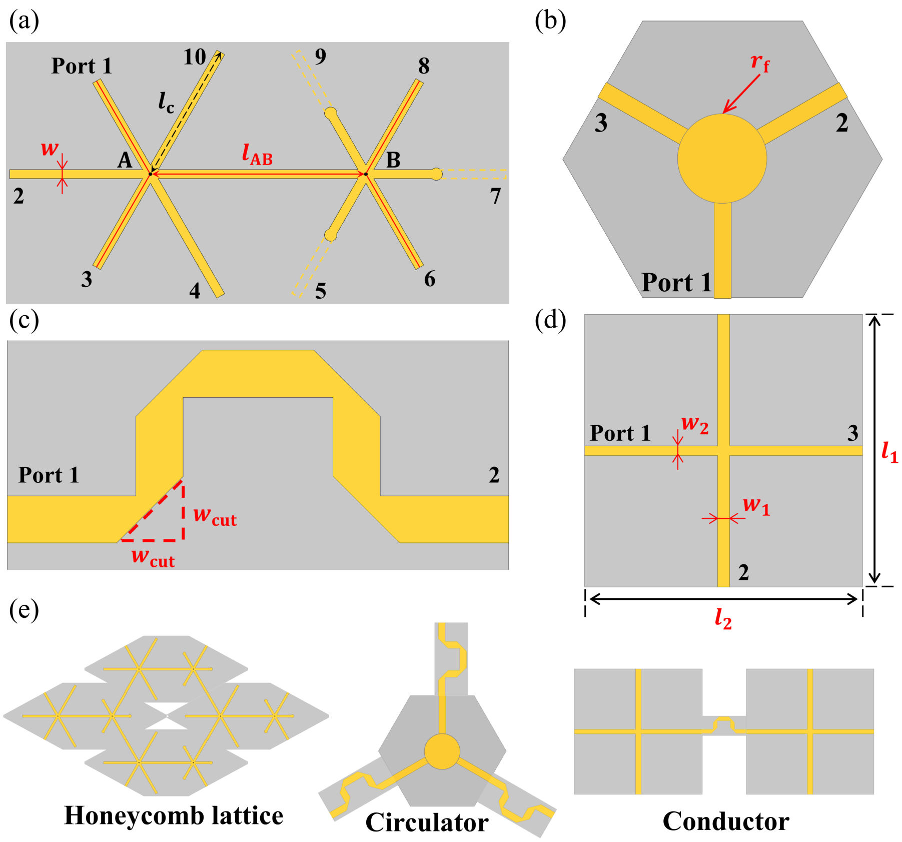


FIG. 16. Schematic of the field-circuit co-simulation. (a)Blocks used to construct honeycomb lattice and connect lattice sites with circulators. (b) Circulators. (c) Blocks used to adjust the electrical length between two sites at a fixed distance. (d) Blocks used for conductors. (e) Examples of assembling the blocks. All the bolcks have undergone microwave electromagnetic simulation to solve the S-parameters among corresponding ports. Then they are assembled into the junction.

52.2 mm. The length of the lines connected to circulators is $l_c = 34.1$ mm. It should noted that, such lines (namely, port 2, 4, 5, 7, 9, 10) are set only for the calculation of S-parameters, which are necessary in the co-simulation. However, when constructing the complete model or in experiment, they can be removed and connect sublattice sites with circulators directly.

Figure 16b is a circulator with the same line width of $w$. Parameters of the ferrite is radius $r_f = 5$ mm, dielectric constant $\varepsilon_f = 37.4$, Saturation magnetization $4\pi M_s = 1800$ Gauss and the external magnetic field $H_z = -2120$ Oe.

Figure 16c shows the right-angle bending design of ML, which is used to achieve variable electrical length between two sites with a fixed spatial distance. The key parameter of this structure is the cutting width $w_{cut} = 1.5w$ mm, which minimizes the reflection caused by impedance changes at corners. In the co-simulation, this structure is used to adjust the phase response of circulators and conductors. For circulators, its electrical length is set to ensure that the phase change of the electromagnetic wave after passing through two of the structures and one circulator is 0. And for conductors, it introduces an additional electrical length of $\pi$ along the direction parallel to the junction.

Figure 16d shows the unit of the rectangular lattice conductor with $w_1 = 2.2$ mm, $w_2 = 1.8$ mm, $l_1 = 49.9$ mm and $l_2 = 50.8$ mm.

S-parameters among the corresponding ports of the four components are separately simulated. Subsequently, the components are utilized to construct the junction model in CST design studio for microwave field-circuit co-simulation. The results are presented as the red squares in Fig. 3b in the main text.

## VII. KWANT SIMULATION

In this section, we firstly introduce the details about simulating the transport of the topological junction with Kwant [18]. Then, in order to realize nearly equivalent scattering properties of a semi-infinite conductor with finite size, the details about imaginary absorbing potential are provided.

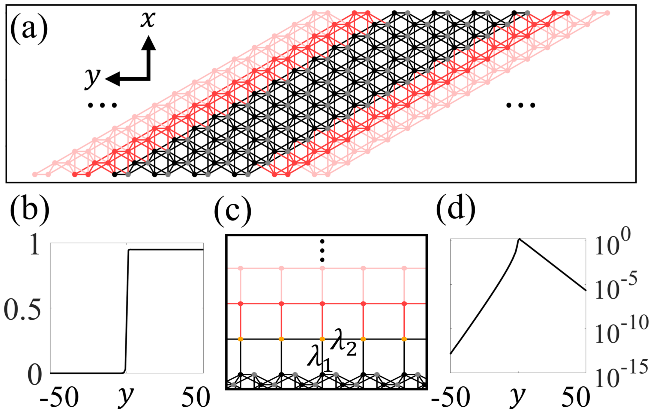


FIG. 17. (a) The Kwant simulation model of Haldane ribbon with armchair boundaries. Black and grey sites represent for sublattice A and B, respectively. Red lattice stands for the infinite extension along both directions of $y$. (b) Response profile of 101 sites on the upper boundary of (a) when excited at the center. (c) The semi-infinite conductor attached to sublattice A of the Haldane ribbon. $\lambda_1$ and $\lambda_2$ are the hopping of the conductor lattice along $x$ and $y$, respectively. (d) Response profile of the same region and excitation as (b) after the attachment of the conductor.

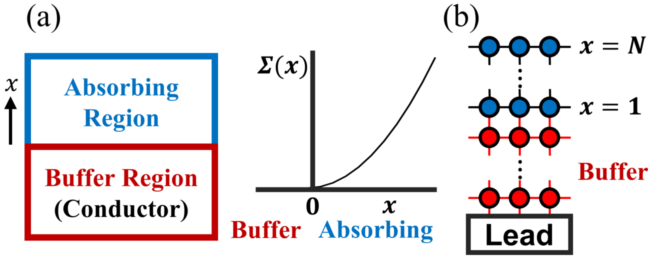


FIG. 18. (a) Schematic of the imaginary potential method. (b) Kwant model used to optimize the controlling parameters. A lead is attached to the bottom to simulate the reflection.

### A. Topological junction

To demonstrate the non-bloch transport of topological insulator–conductor junction, Kwant, a open source Python package, is adopted. Firstly, the simulation model of a Haldane ribbon with armchair boundaries is constructed (Fig. 17a). The corresponding hoppings are set to be $t_1 = t_2 = 1$. Transport properties of the topological insulator are simulated by calculating the Green's function of the upper side for 101 lattice sites. When excited at the center, the response of all sites is depicted as Fig. 17b, which represents for the chiral boundary state of Haldane model. Based on the Haldane ribbon, a semi-infinite conductor with square lattice is attached to sublattice A to construct the junction (Fig. 17c). Hopping parameters of the conductor lattice are set to be $\lambda_1 = 1$ and $\lambda_2 = -0.9$. Transport properties of the junction are simulated in the same way and at the same region as above. The corresponding response is shown as Fig. 17d. In Fig. 17b, waves cannot propagate along $-y$ because of the boundary state being anticlockwise. However, in Fig. 17d, waves decay exponentially at different rates in different directions, which represents for the non-bloch transport and can be attributed to the non-Hermiticity introduced by the Hermitian semi-infinite conductor.

### B. Imaginary absorbing potential

Constructing the junction needs for a semi-infinite conductor that is impractical for experimental setup. Therefore, imaginary potential method [19, 20] is adopted on a finite conductor to realize equivalent effects as a semi-infinite one. As shown in Fig. 18a, the method consists of two regions. In absorbing region, imaginary onsite potential is introduced to the lattice sites to absorb the waves propagating towards the end. Moreover, a buffer region is used to extend the propagation time of the ineluctable backscattering wave so that it would not influence the transportation of the topoligical junction in certain simulation time. According to Ref. [19], a polynomial form of imaginary onsite potential is adopted:

$$\Sigma(x) = i(n+1)Ax^n, \tag{59}$$

where $n$ and $A$ are controlling parameters, and $x$ is the order number counted from the start point of the absorbing region (Fig. 18b). Generally, the values of imaginary potential should be large enough so that the waves can be absorbed within a region as small as possible. However, sharp change of the values from one point to the next causes backscattering that weakens the absorption. Thus, the actual problem is the optimization about controlling parameters $n$, $A$, and the length of the buffer and absorbing region in $x$. To obtain appropriate parameters, a finite square lattice with imaginary onsite potential according to Eq. 59 is constructed in Kwant (Fig. 18b). The number of sites in each layer is 15 according to the experimental design and the length of the buffer region in $x$ is 5 layers. A lead is attached to the lattice to simulate the reflection. At a fixed length $N$ of the absorbing region, parameter sweep of $n$ and $A$ is performed to minimize the reflection. The same process is executed for different values of $N$. Finally, for circuit experiment parameters of $\lambda_1 = -1$, $\lambda_2 = 0.1$, we choose the controlling parameters as $N = 5$, $n = 1.8$ and $A = 0.025$, with a reflectivity less than 1%.

## VIII. EXPERIMENTAL DETAILS

In this section, we give details about the experimental setup of the circuits topological junction. The junction can be divided into two parts, namely, topological insulator circuits and conductor circuits as shown in Fig. 19a. Both of them are manufactured through printed circuit boards (PCBs), and then connected together.

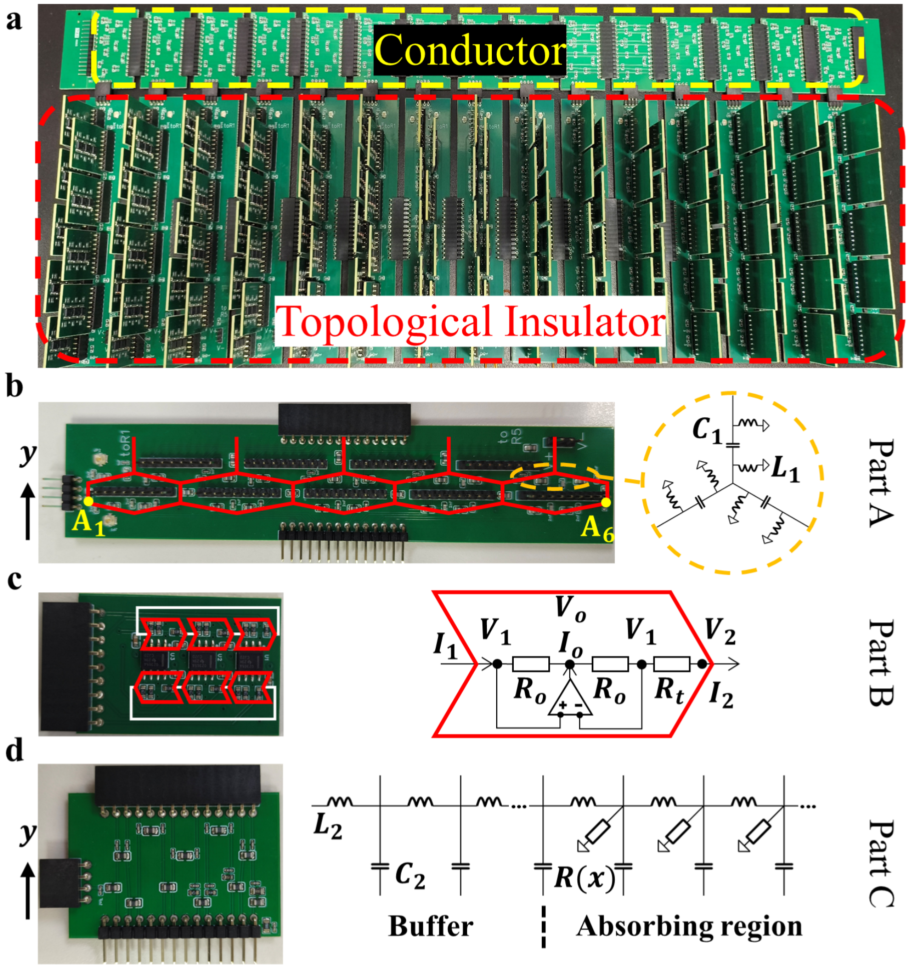


FIG. 19. Experimental setup of the circuit topological junction. (a) The junction consists of topological insulator and conductor. (b) Part A is used to construct the honeycomb lattice. The inset shows the configuration of LCL resonance couple. In experiment, the voltage on site $A_1$ is measured. (c) Part B realizes the non-reciprocal coupling $t_2$ within a single hexagon, which consists of six INICs. (d) Part C constructs the conductor with buffer and absorbing region.

### A. Circuit realization of Haldane model

The circuit Haldane model consists of two kinds of PCBs, corresponding to the honeycomb lattice and the next-nearest-neighbor (NNN) hoppings within a single hexagon unit, respectively. Figure 19b shows the PCB of honeycomb lattice, which is referred to as part A for convenience. The nearest-neighbor hopping amplitude of $t_1 = 1$ is achieved through an inductor-capacitor-inductor (LCL) resonance couple, with $L_1 = 3.5\ \mu$H and $C_1 = 1$ nF. Figure 19c shows the PCB of NNN hoppings (referred to as part B). We use three two-gate operational amplifiers (OPA2365, Texas Instruments) in each to construct six negative impedance converters with current inversion (INICs). The structure of INIC is shown on the right of Fig. 19c. An INIC leads to $-I_1 = I_2$ [21], which means a negative resistance $-R_t$ from node 1 to node 2 and a positive resistance $R_t$ from node 2 to node 1, thus introducing the non-reciprocal coupling.

The NNN hopping amplitude of $t_2 = 1/6$ is achieved through a resistor of $R_t = 348\,\Omega$ as the effective resistor of an INIC. When constructing the Haldane model, 15 pieces of part A are connected along $y-$direction, then 131 pieces of part B are inserted on them. Additionally, the site $A_6$ of each part A is grounded with a resistor of $27\,\Omega$ in order to eliminate the reaching voltage signals through the edge state, thus simulating the infinite length along $y-$direction.

The tolerance of resistors, capacitors and inductors are 0.1%, 1%, and 5%, respectively.

### B. Circuit realization of the semi-infinite conductor

Figure 19d shows the PCB of the conductor (referred to as part C). It consists of buffer (5 layers) and absorbing region (5 layers). The corresponding parameters of circuit components are $L_2 = 3.5\ \mu$H (for $\lambda_1 = -1$), $C_2 = 100$ pF (for $\lambda_2 = 0.1$), $R(6) = 820\,\Omega$, $R(7) = 237\,\Omega$,

$R(8) = 115\,\Omega$, $R(9) = 68\,\Omega$, and $R(10) = 45.3\,\Omega$. Additionally, each node of absorbing region is also grounded with a capacitor of 470 pF to adjust the onsite potential. When constructing the topological junction, 15 pieces of part C are connected along $y-$direction, and then inserted to the top edge of the Haldane circuit.

The tolerance of resistors, capacitors and inductors are 0.1%, 1%, and 5%, respectively.

### C. Measuring of the non-Bloch transport

Before measuring, a DC power supply (E36311A, Keysight) is connected to corresponding electrodes on the PCBs to supply the operational amplifiers and activate the INICs. Subsequently, a waveform generator (33220A, Agilent) delivering a 2.7 MHz sinusoidal signal is connected to site $A_1$ of the 14th part A as the excitation source. This signal is simultaneously routed a lock-in amplifier (HF2LI, Zurich Instruments) as a reference for high-resolution detection.

The propagation characteristics along the negative $y-$direction of the junction are measured by sequentially measuring voltage signals at $A_1$ from the 13th to the 4th part A using the lock-in amplifier. Conversely, the positive $y-$direction propagation are determined by exciting $A_1$ of the 2nd part A and measuring responses from the 3rd to the 12th. The amplitude of all the acquired signals are normalized to the source.

Notably, the frequency-locking capability of the lock-in amplifier enables selective retention of target signals, namely, signals with the same frequency as the excitation, while effectively suppressing extraneous noise of the setup and offset voltage of the operational amplifiers. This methodology facilitates reliable detection of weak signals at the sub-microvolt level.


[1] S. Datta, *Electronic transport in mesoscopic systems* (Cambridge university press, 1997).

[2] A. Alase, E. Cobanera, G. Ortiz, and L. Viola, Exact solution of quadratic fermionic hamiltonians for arbitrary boundary conditions, Phys. Rev. Lett. **117**, 076804 (2016).

[3] E. Cobanera, A. Alase, G. Ortiz, and L. Viola, Exact solution of corner-modified banded block-toeplitz eigensystems, J. Phys. A: Math. Theor. **50**, 195204 (2017).

[4] A. Alase, E. Cobanera, G. Ortiz, and L. Viola, Generalization of bloch's theorem for arbitrary boundary conditions: Theory, Phys. Rev. B **96**, 195133 (2017).

[5] V. Kaladzhyan and C. Bena, Obtaining majorana and other boundary modes from the metamorphosis of impurity-induced states: Exact solutions via the t-matrix, Phys. Rev. B **100**, 081106 (2019).

[6] S. Pinon, V. Kaladzhyan, and C. Bena, Surface green's functions and boundary modes using impurities: Weyl semimetals and topological insulators, Phys. Rev. B **101**, 115405 (2020).

[7] Y. Hatsugai, Chern number and edge states in the integer quantum hall effect, Phys. Rev. Lett. **71**, 3697 (1993).

[8] V. Dwivedi and V. Chua, Of bulk and boundaries: Generalized transfer matrices for tight-binding models, Phys. Rev. B **93**, 134304 (2016).

[9] R. S. K. Mong and V. Shivamoggi, Edge states and the bulk-boundary correspondence in dirac hamiltonians, Phys. Rev. B **83**, 125109 (2011).

[10] M. Wimmer, *Quantum transport in nanostructures: From computational concepts to spintronics in graphene and magnetic tunnel junctions*, Phd thesis, University of Regensburg, Regensburg (2009).

[11] D. H. Lee and J. D. Joannopoulos, Simple scheme for surface-band calculations. ii. the green's function, Phys. Rev. B **23**, 4997 (1981).

[12] M. Wu, Q. Zhao, L. Kang, M. Weng, Z. Chi, R. Peng, J. Liu, D. H. Werner, Y. Meng, and J. Zhou, Evidencing non-bloch dynamics in temporal topolectrical circuits, Phys. Rev. B **107**, 064307 (2023).

[13] M. Wu, M. Weng, Z. Chi, Y. Qi, H. Li, Q. Zhao, Y. Meng, and J. Zhou, Observing relative homotopic degeneracy conversions with circuit metamaterials, Phys. Rev. Lett. **132**, 016605 (2024).

[14] D. Youla, L. Castriota, and H. Carlin, Bounded real scattering matrices and the foundations of linear passive network theory, IRE Transactions on Circuit Theory **6**, 102 (1959).

[15] J. Helszajn, Waveguide and stripline 4-port single-junction circulators (short papers), IEEE Transactions on Microwave Theory and Techniques **21**, 630 (1973).

[16] J. Helszajn, M. McKay, and I. Macfarlane, Complex gyrator circuit of 4-port single junction circulator, IEEE microwave and wireless components letters **14**, 40 (2004).

[17] J. Helszajn, The adjustment of the m-port single-junction circulator, IEEE Transactions on Microwave Theory and Techniques **18**, 705 (1970).

[18] C. W. Groth, M. Wimmer, A. R. Akhmerov, and X. Waintal, Kwant: a software package for quantum transport, New Journal of Physics **16**, 063065 (2014).

[19] J. Weston and X. Waintal, Linear-scaling source-sink algorithm for simulating time-resolved quantum transport and superconductivity, Phys. Rev. B **93**, 134506 (2016).

[20] T. Kloss, J. Weston, B. Gaury, B. Rossignol, C. Groth, and X. Waintal, Tkwant: a software package for time-dependent quantum transport, New Journal of Physics **23**, 023025 (2021).

[21] T. Hofmann, T. Helbig, C. H. Lee, M. Greiter, and R. Thomale, Chiral voltage propagation and calibration in a topolectrical chern circuit, Phys. Rev. Lett. **122**, 247702 (2019).
